# Supplementary material for: Small Models Are (Still) Effective Cross-Domain Argument Extractors
Source: arXiv:2404.08579 source file (2024-04-12)
Supplement: Supplementary file 1 [file additional_results.tex]

% This appendix contains 

% \begin{table*}[t]
%     \centering
%     \begin{tabular}{l|c|c|cccccc}
%     \toprule
%         Model & Method & Source Dataset & ACE & ERE-L & ERE-R & FAMuS & RAMS & WikiEvents \\
%     \midrule
%         \multirow{6}{*}{BART} & \multirow{6}{*}{TI} & ACE & \textbf{57.54} & 37.33 & 28.68 & 15.56 & 20.23 & \phantom{0}9.35 \\
%         & & ERE-L & 27.08 & \textbf{60.62} & \underline{45.26} & 14.33 & 19.91 & 13.79 \\
%         & & ERE-R & \underline{43.76} & \underline{56.78} & \textbf{61.14} & 16.49 & 22.04 & 15.79 \\
%         & & FAMuS & 29.56 & 27.06 & 20.06 & \textbf{38.43} & 19.81 & \phantom{0}6.52 \\
%         & & RAMS & 24.94 & 33.60 & 25.58 & 15.96 & \textbf{46.08} & \underline{24.94} \\
%         & & WikiEvents & 25.38 & 29.60 & 24.22 & \phantom{0}9.85 & 24.43 & \textbf{57.54} \\
%         \midrule
%         \multirow{6}{*}{BART} & \multirow{6}{*}{QA} & ACE & \textbf{63.05} & 39.53 & 44.97 & 24.82 & 29.77 & 18.86 \\
%         & & ERE-L & 21.31 & \textbf{63.63} & 34.92 & 13.86 & 22.59 & 18.93 \\
%         & & ERE-R & 36.45 & 52.06 & \textbf{57.70} & \underline{27.34} & \underline{32.72} & 23.52 \\
%         & & FAMuS & 34.62 & 34.77 & 30.51 & \textbf{43.37} & 27.59 & \phantom{0}9.41 \\
%         & & RAMS & 26.68 & 28.64 & 31.25 & 19.07 & \textbf{44.08} & \underline{27.35} \\
%         & & WikiEvents & 19.22 & 24.97 & 24.97 & \phantom{0}9.27 & 27.16 & \textbf{54.93} \\
%         \midrule
%         GPT-3.5 & \multirow{2}{*}{QA} & - & 27.55 & 27.50 & 18.42 & 26.80 & 22.67 & 10.46 \\ 
%         GPT-4 & & - & & & & & & \\ 
%     \bottomrule
%     \end{tabular}
%     \caption{Results for the same experimental setup as in \autoref{tab:results-flan-t5}, but using Flan-T5 \citep{chung-etal-2022-scaling} in lieu of BART. Results for GPT-3.5 and GPT-4 are copied from \autoref{tab:results-flan-t5} for ease of reference.}
%     \label{tab:results-bart}
% \end{table*}

% \begin{table*}
%     \centering
%     \adjustbox{max width=\textwidth}{
%     \begin{tabular}{l|l}
%     \toprule
%          & Event Types \\
%     \midrule
%         ACE & Life.Divorce, Conflict.Demonstrate, Justice.Fine, Justice.Arrest-Jail, Business.Start-Org, \\
%         & Business.End-Org, Justice.Charge-Indict, Justice.Sentence, Personnel.End-Position, Movement.Transport \\
%         \midrule
%         ERE-L & Business.End-Org, Personnel.Nominate, Conflict.Demonstrate, Justice.Arrest-Jail \\
%         & Life.Be-Born, Life.Die, Life.Marry, Life.Divorce, Business.Start-Org, Conflict.Attack \\
%         \midrule
%         ERE-R & Manufacture.Artifact, Business.Start-Org, Business.Merge-Org, Life.Be-Born, Life.Marry \\
%         & Justice.Convict, Justice.Arrest-Jail, Conflict.Attack, Justice.Execute, Justice.Transport-Person \\
%         \midrule
%         RAMS & Contact.Collaborate.Meet, Government.Agreements.ViolateAgreement, Life.Injure.IllnessDegradationHungerThirst, \\
%         & Conflict.Attack.AirStrikeMissileStrike, Government.Formation.StartGPE, \\ & Movement.TransportArtifact.SendSupplyExport, Conflict.Demonstrate.MarchProtestPoliticalGathering, \\ & Contact.CommandOrder.Unspecified, Movement.TransportPerson.Fall, Movement.TransportArtifact.Hide \\
%         \midrule
%         WikiEvents & Justice.InvestigateCrime.Unspecified, Contact.RequestCommand.Unspecified, Medical.Intervention.Unspecified \\
%         & Transaction.ExchangeBuySell.Unspecified, Cognitive.IdentifyCategorize.Unspecified, Justice.ArrestJailDetain.Unspecified \\
%         & Life.Die.Unspecified, Justice.ChargeIndict.Unspecified, Contact.Contact.Broadcast, Conflict.Attack.DetonateExplode \\
%     \bottomrule
%     \end{tabular}}
%     \caption{The 10 event types in each target ontology for which the FAMuS-trained QA model obtains \textbf{highest} argument $\text{F}_1$ score (ordered highest-to-lowest).}
%     \label{tab:type_breakdown_highest}
% \end{table*}

% \begin{table*}
%     \centering
%     \adjustbox{max width=\textwidth}{
%     \begin{tabular}{l|l}
%     \toprule
%          & Event Types \\
%     \midrule
%         ACE & Justice.Release-Parole, Justice.Acquit, Business.Declare-Bankruptcy, Life.Marry, Justice.Sue \\
%         & Contact.Phone-Write, Conflict.Attack, Life.Be-Born, Justice.Execute, Life.Die \\
%         \midrule
%         ERE-L & Justice.Appeal, Contact.Meet, Justice.Release-Parole, Justice.Charge-Indict, Life.Injure \\
%         & Transaction.Transfer-Money, Justice.Convict, Justice.Acquit, Personnel.Start-Position, Personnel.End-Position \\
%         \midrule
%         ERE-R & Justice.Release-Parole, Life.Divorce, Life.Injure, Personnel.End-Position, Transaction.Transfer-Money \\
%         & Personnel.Start-Position, Contact.Meet, Transaction.Transaction, Justice.Appeal, Conflict.Demonstrate \\
%         \midrule
%         RAMS & Conflict.Attack.Hanging, Contact.Collaborate.Unspecified, Contact.CommandOrder.Meet, Contact.FuneralVigil \\
%         & Contact.Negotiate.Unspecified, Disaster.FireExplosion.FireExplosion, Life.Die.NonViolentDeath \\
%         & Life.Injure.IllnessDegradationPhysical, Manufacture.Artifact.CreateManufacture, Movement.TransportArtifact.ReceiveImport \\
%         \midrule
%         WikiEvents & DamageDestroyDisableDismantle.Damage, DamageDestroyDisableDismantle.Destroy, \\
%         & DamageDestroyDisableDismantle.DisableDefuse, DamageDestroyDisableDismantle.Dismantle, \\
%         & ArtifactExistence.ManufactureAssemble.Unspecified, Cognitive.Inspection.SensoryObserve \\
%         & Cognitive.Research.Unspecified, Conflict.Demonstrate.Unspecified \\
%         & Contact.Contact.Correspondence, Contact.Contact.Meet \\
%     \bottomrule
%     \end{tabular}}
%     \caption{The 10 event types in each target ontology for which the FAMuS-trained QA model obtains \textbf{lowest} argument $\text{F}_1$ score (ordered lowest-to-highest).}
%     \label{tab:type_breakdown_lowest}
% \end{table*}
